# Supplementary material for: Ground and excited states of doubly open-shell nuclei from ab initio valence-space Hamiltonians
Source: arXiv:1511.02802 source file (2016-05-09)

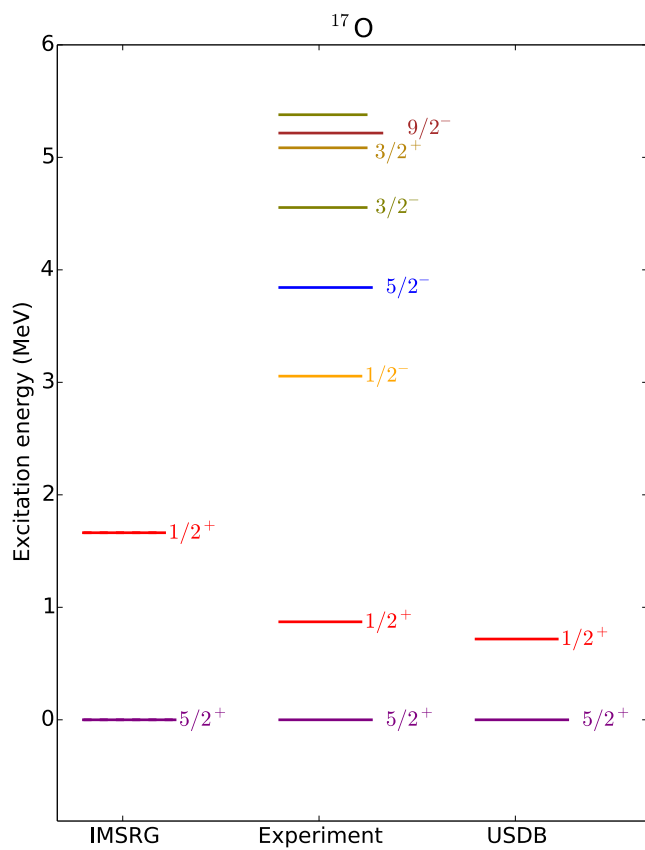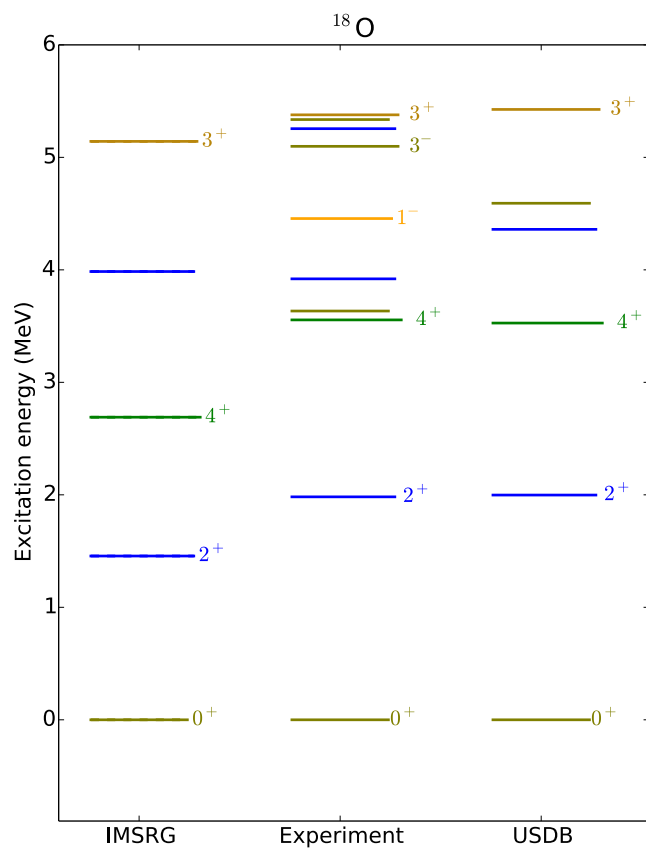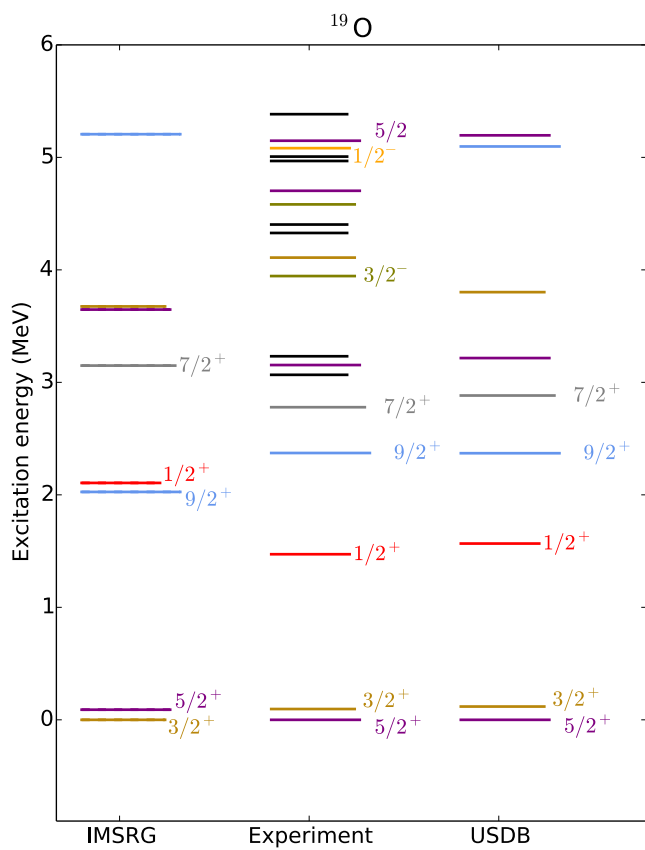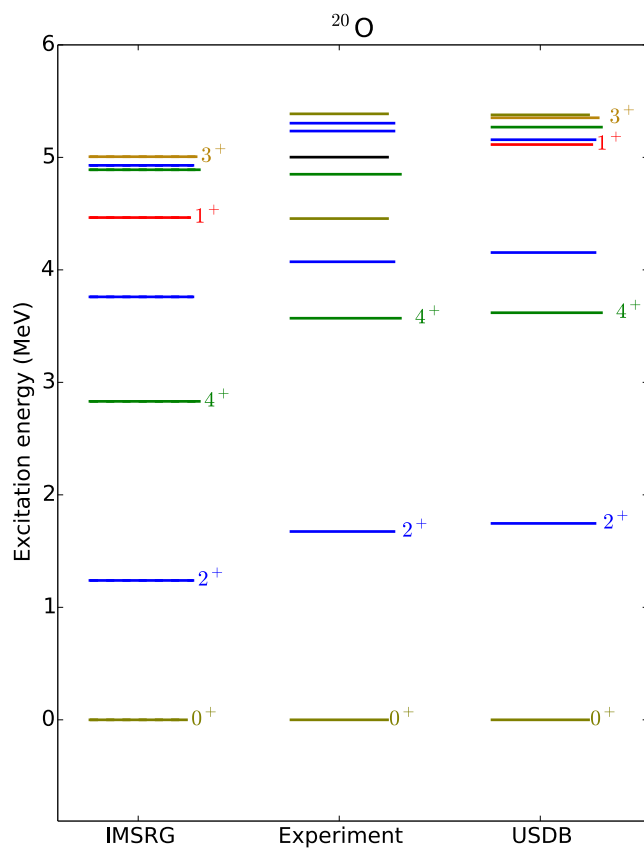

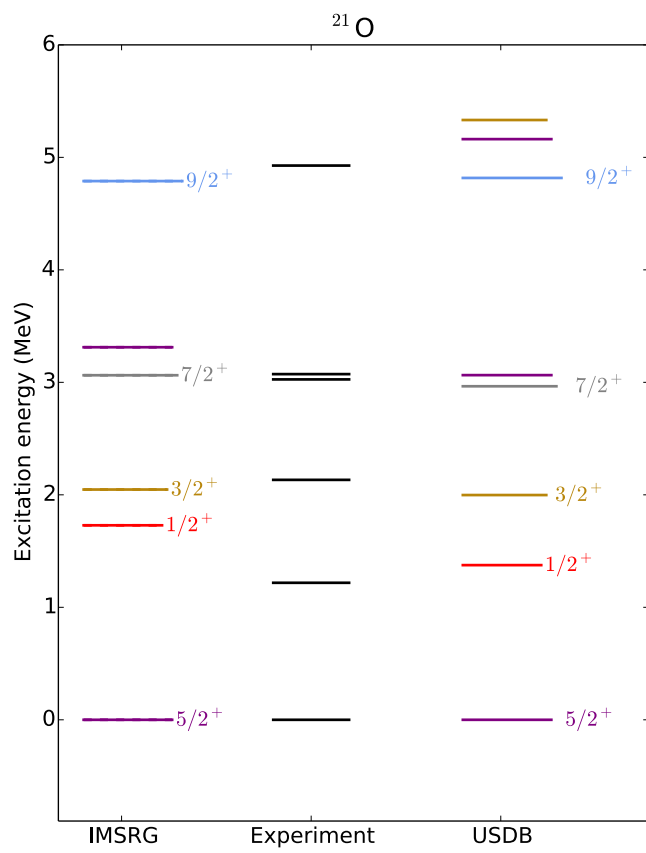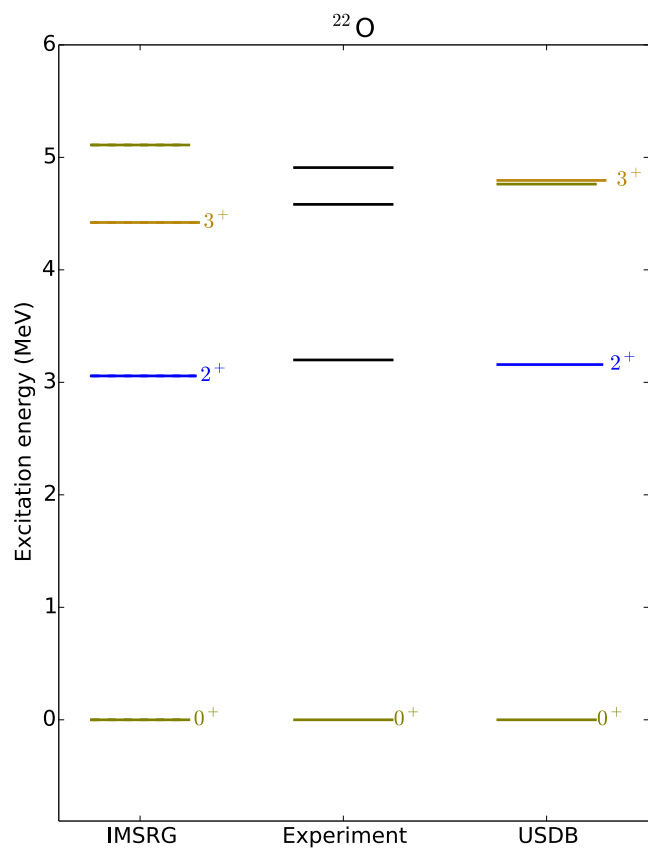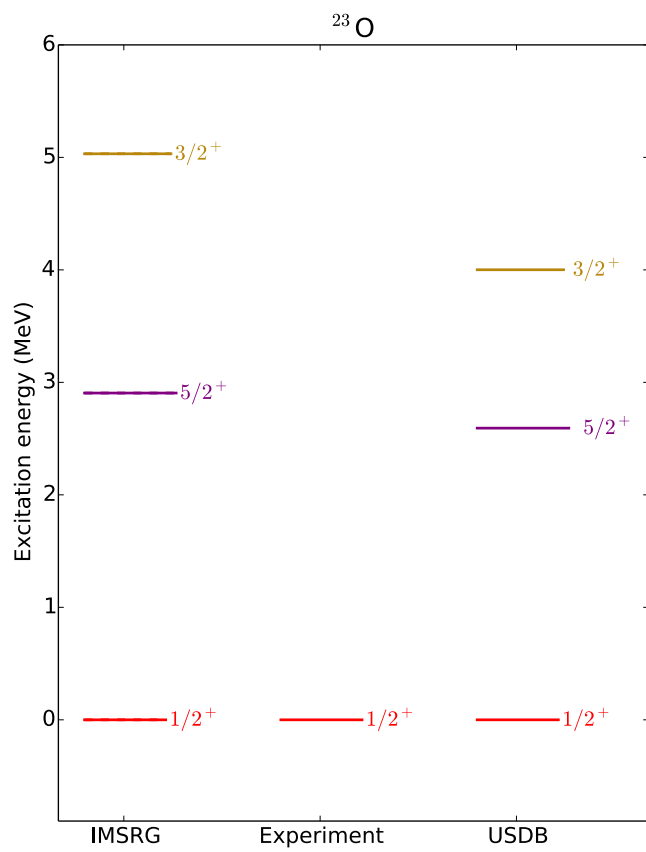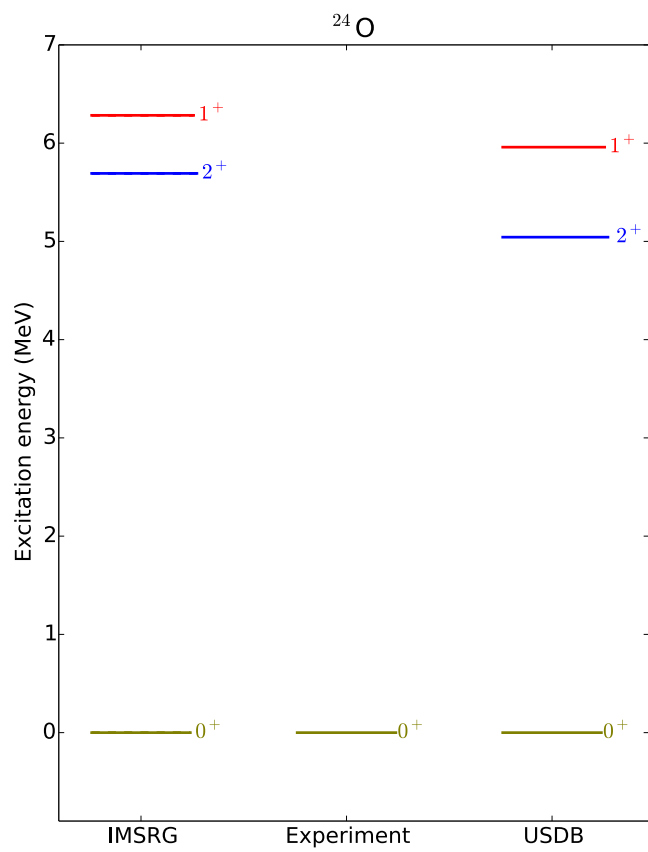

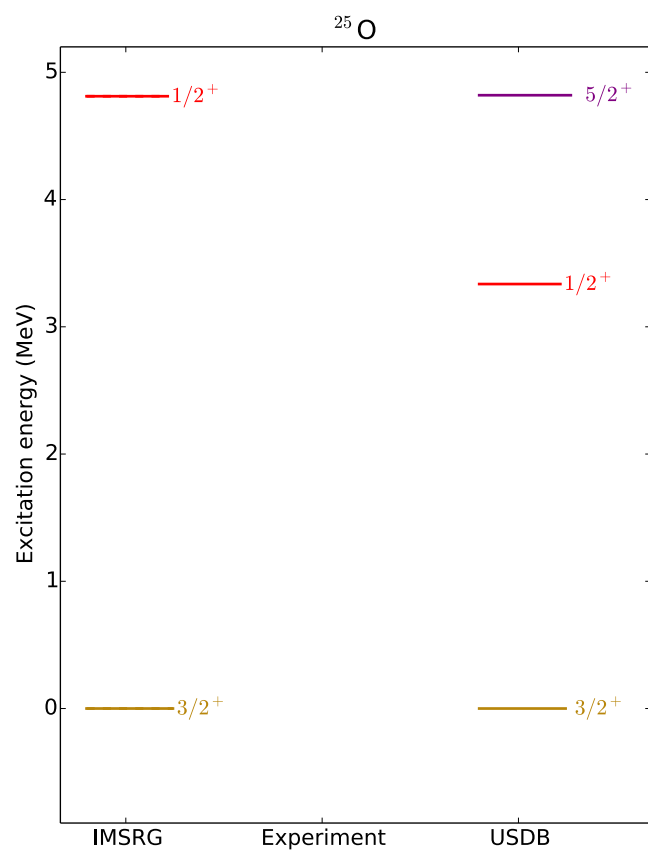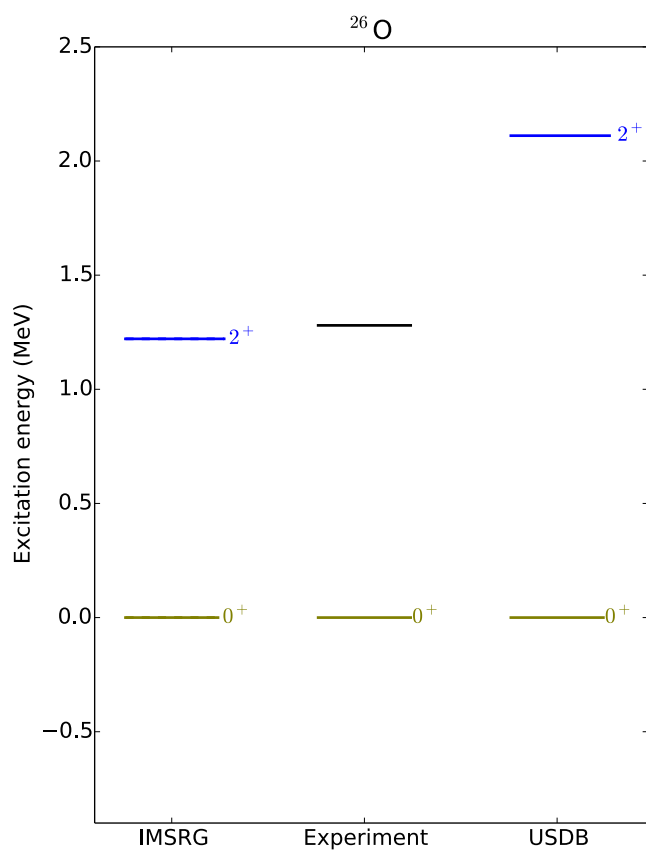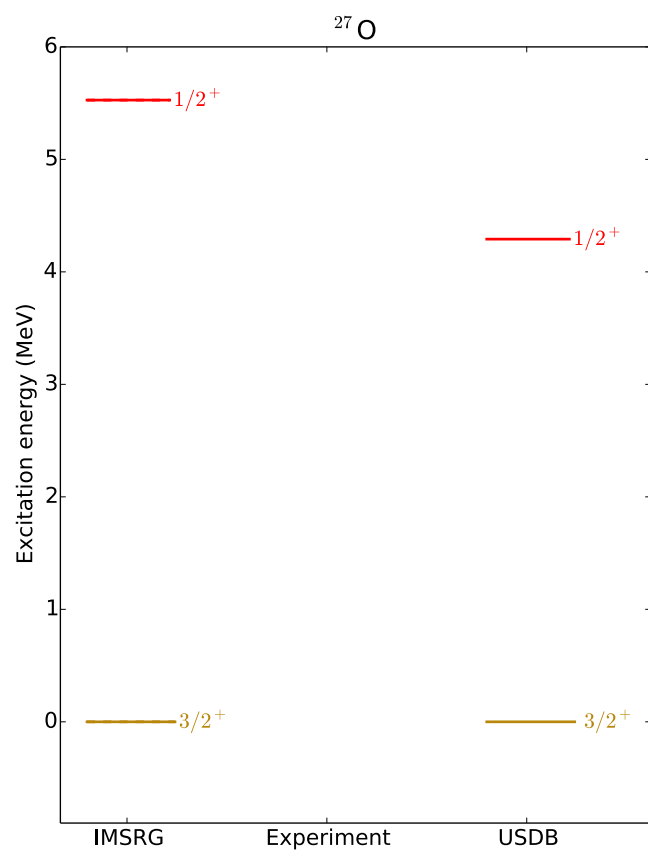

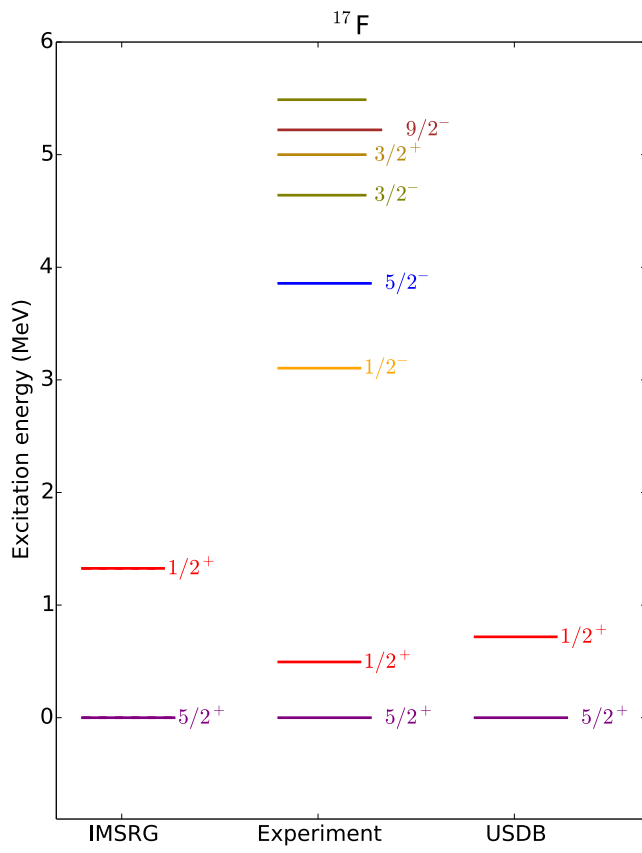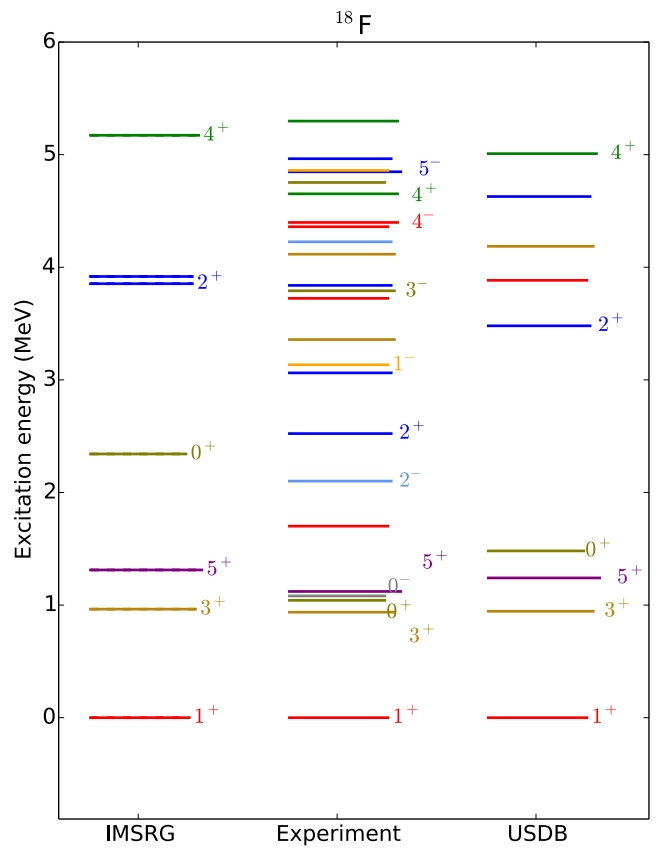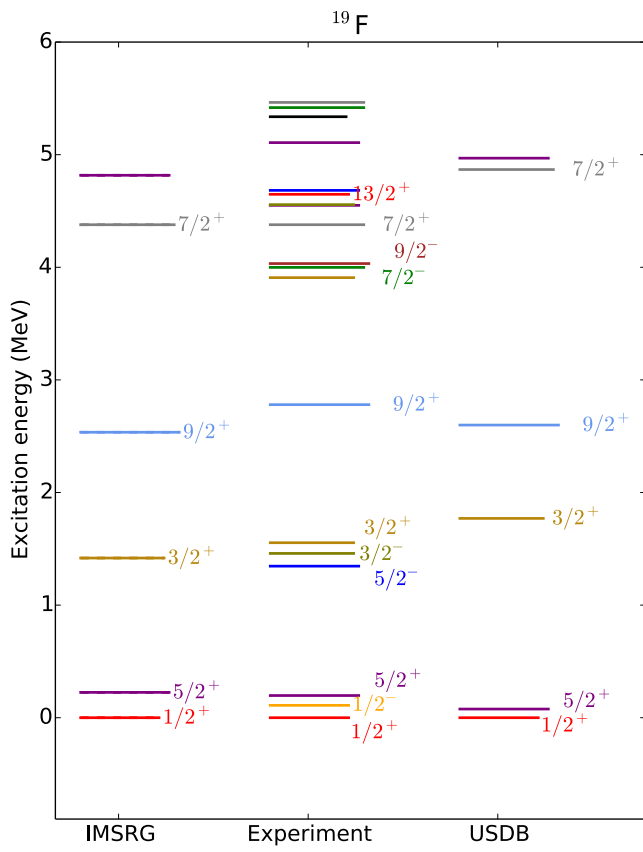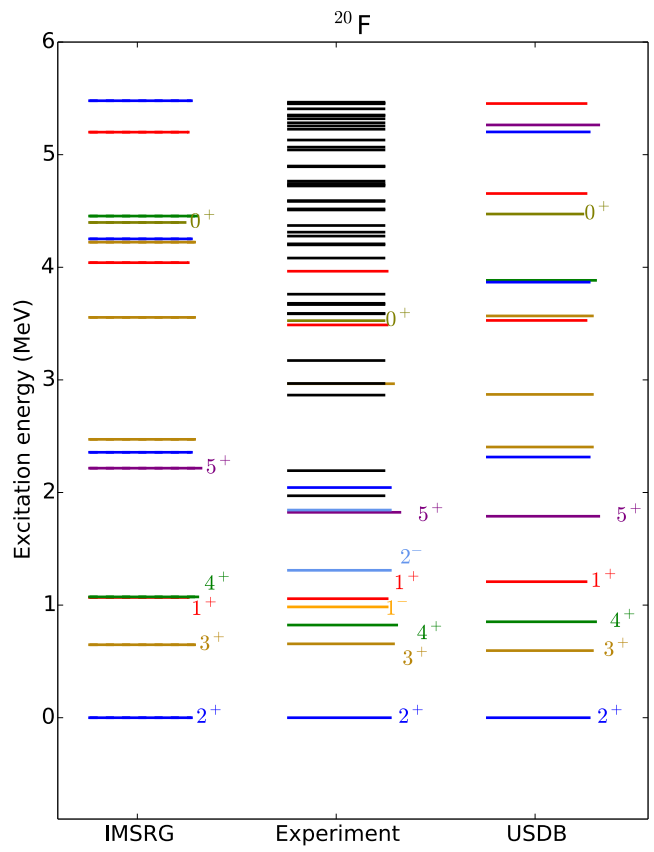

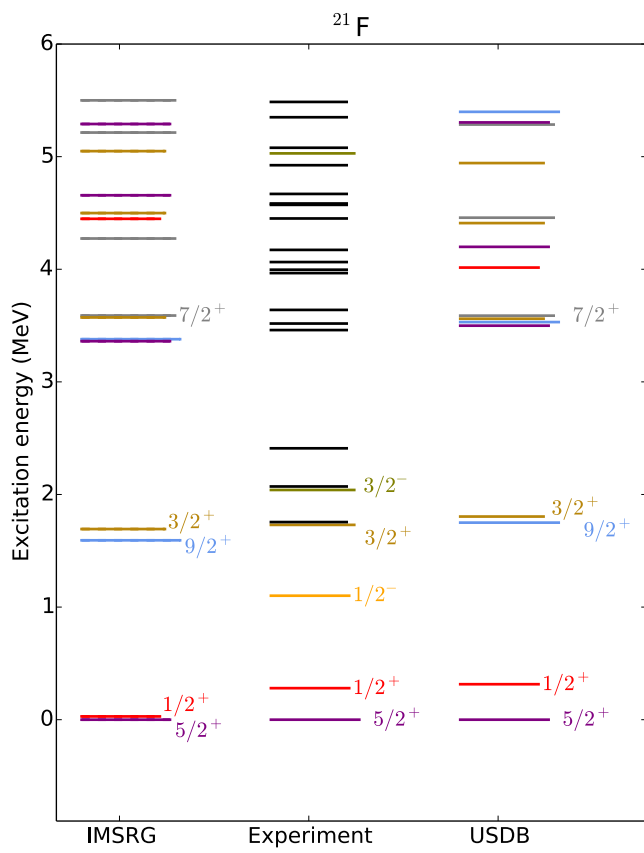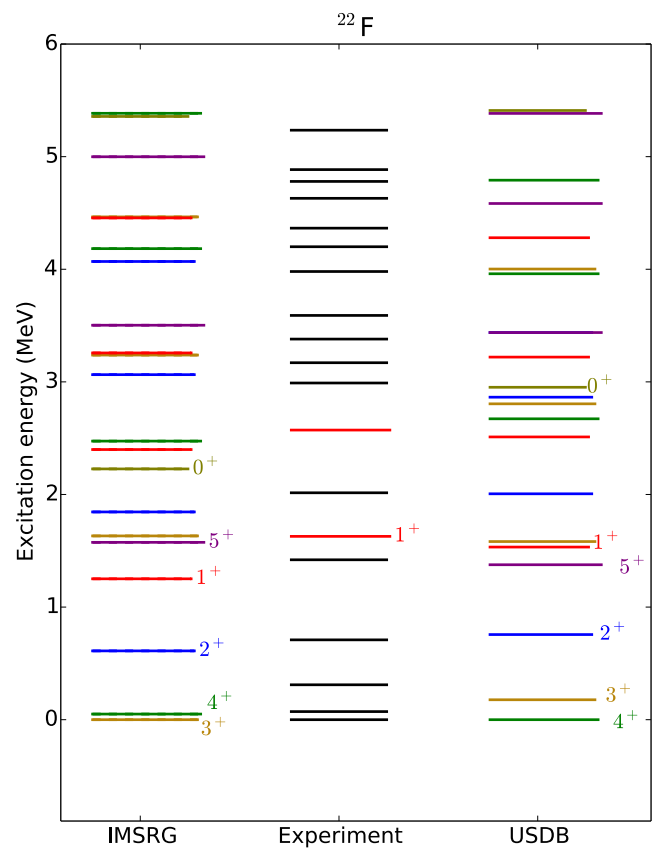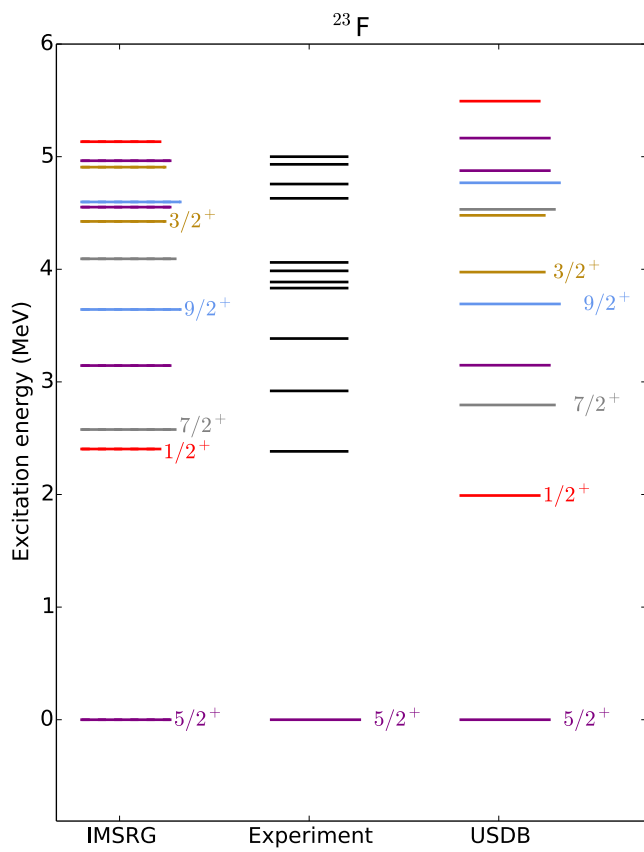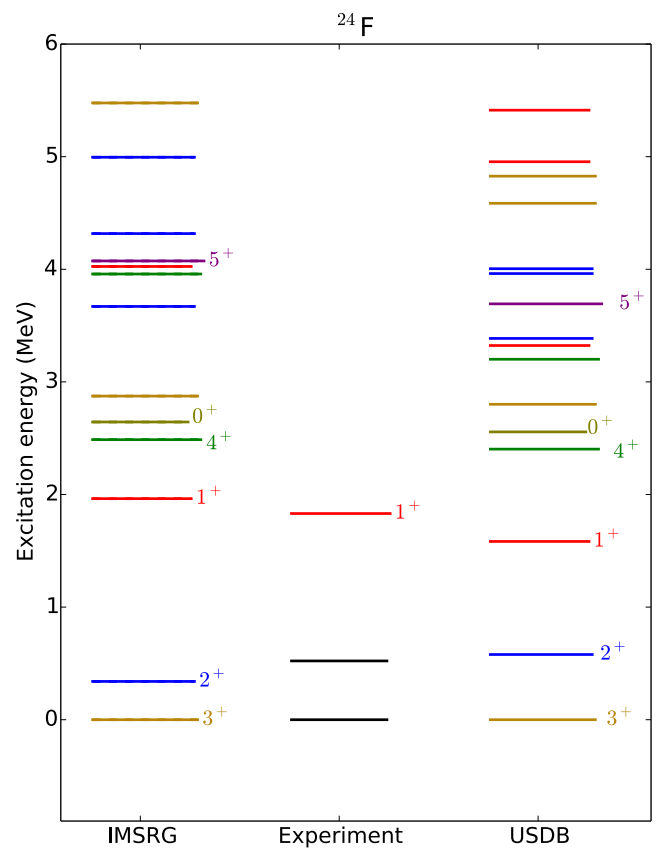

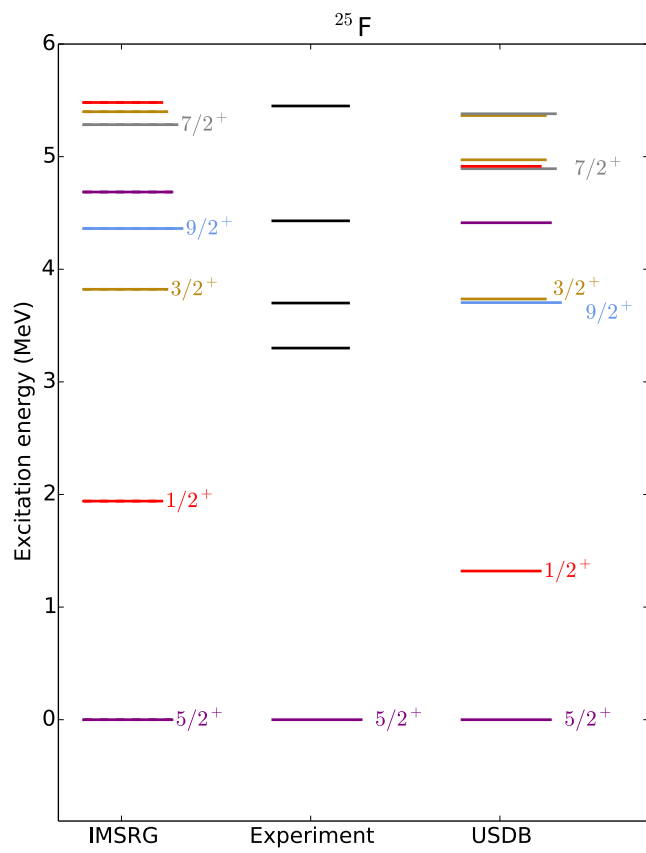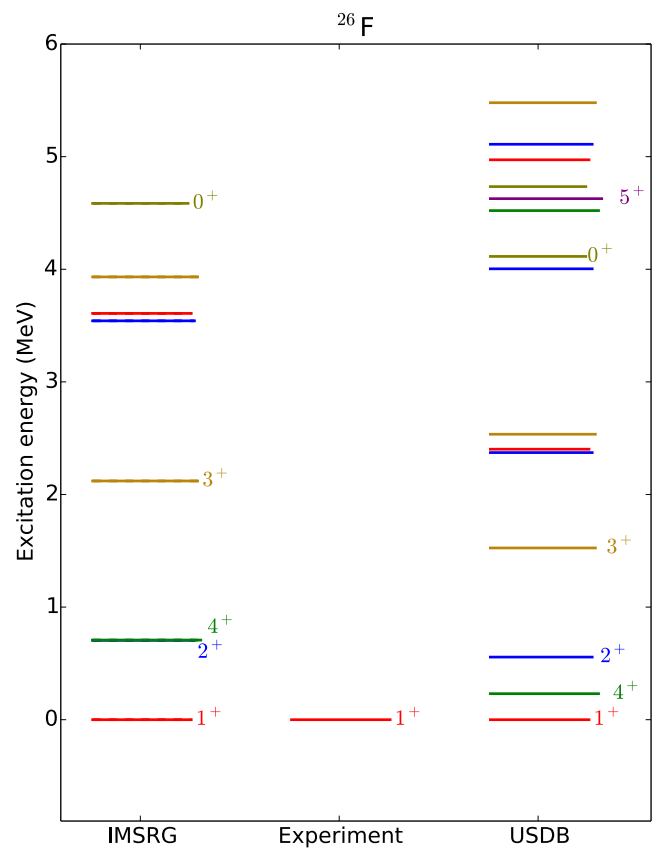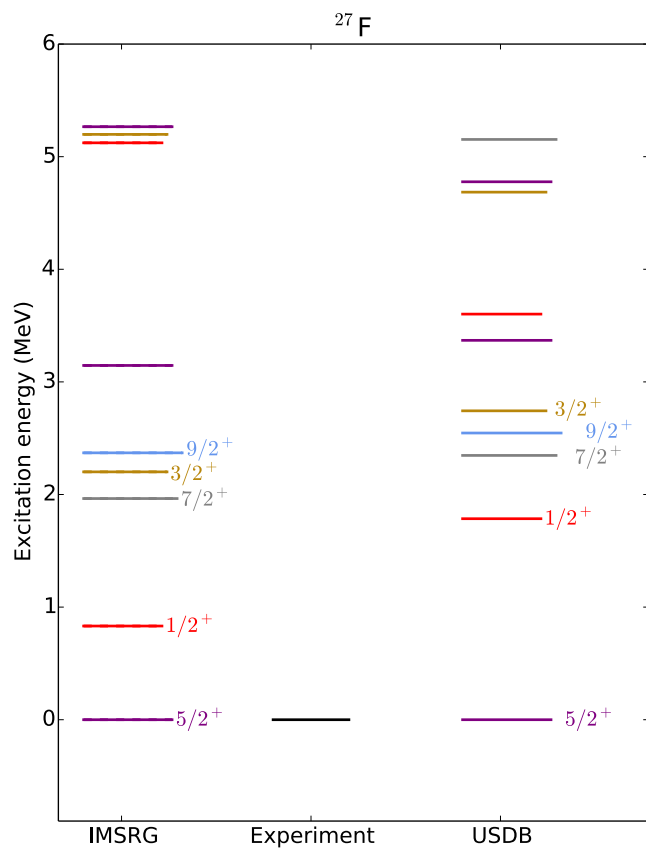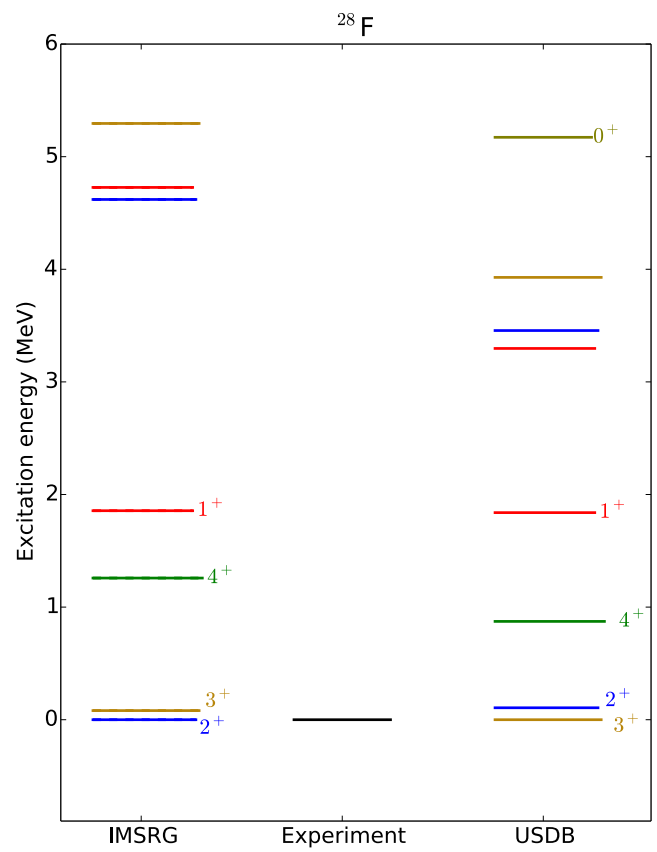

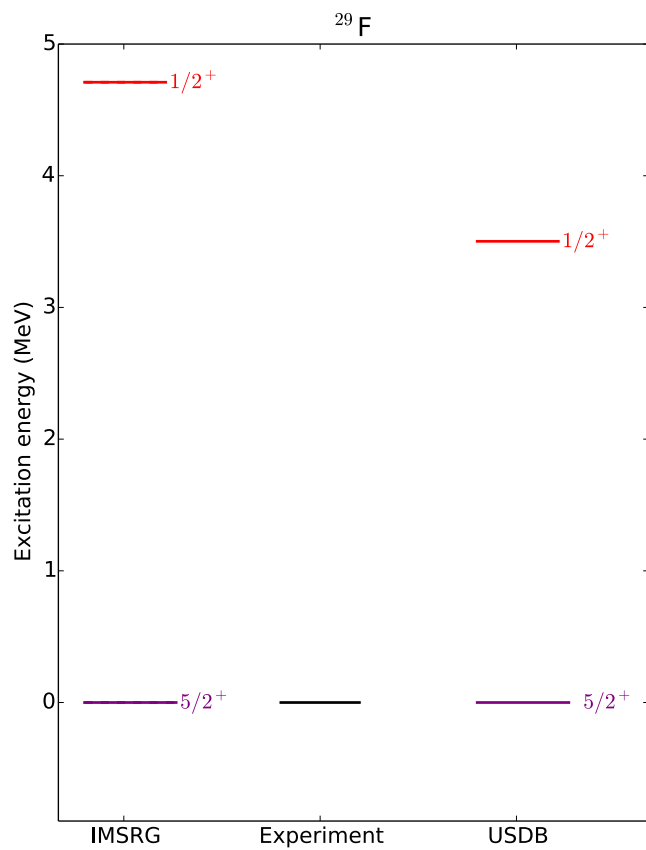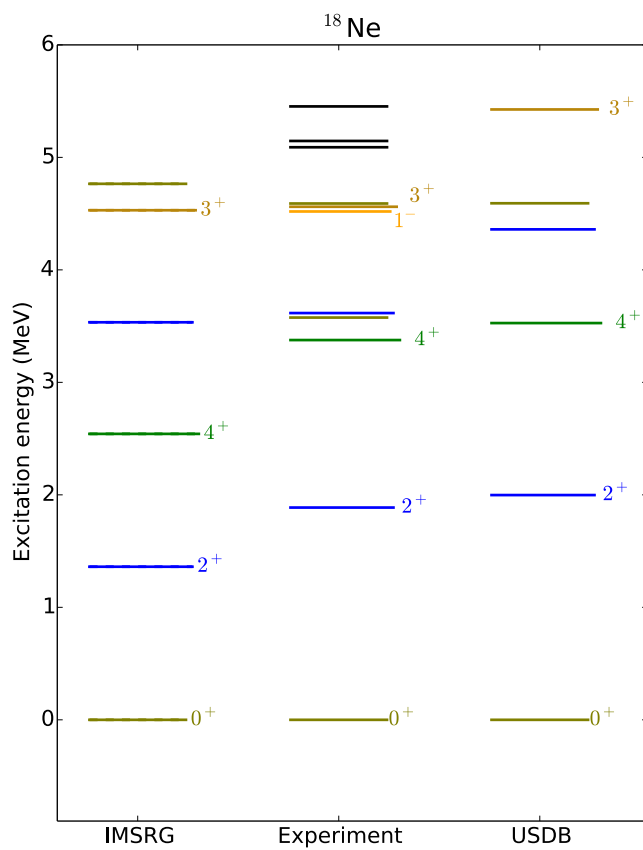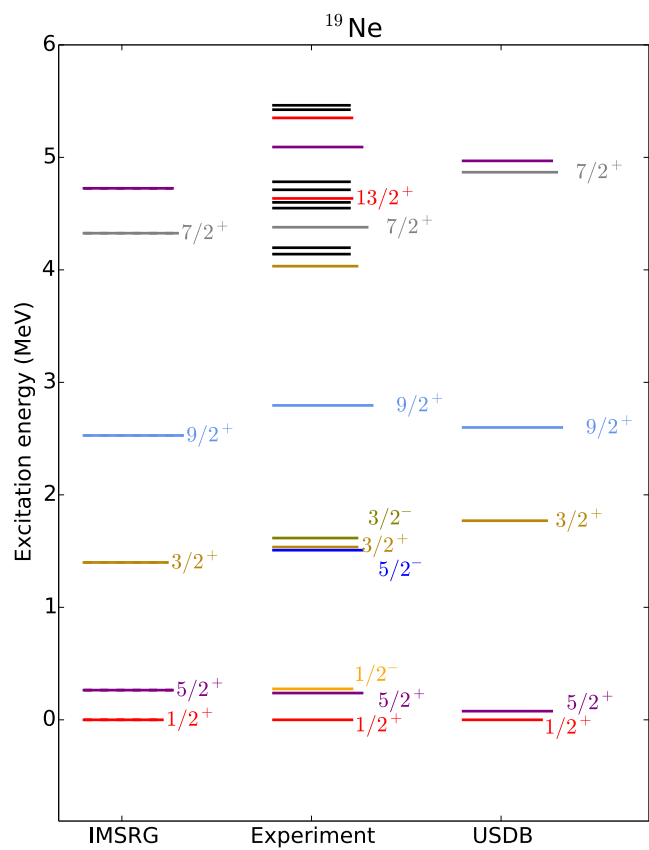

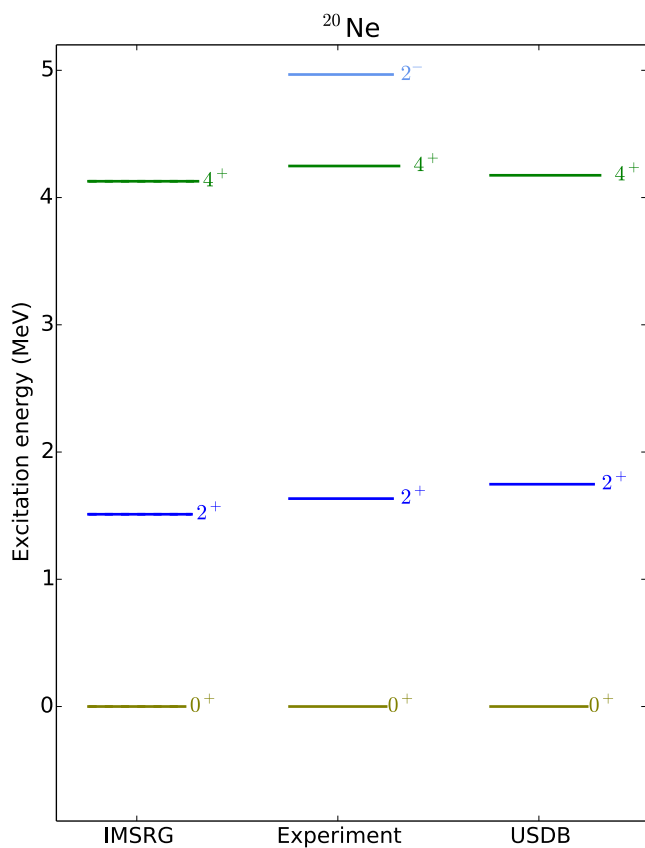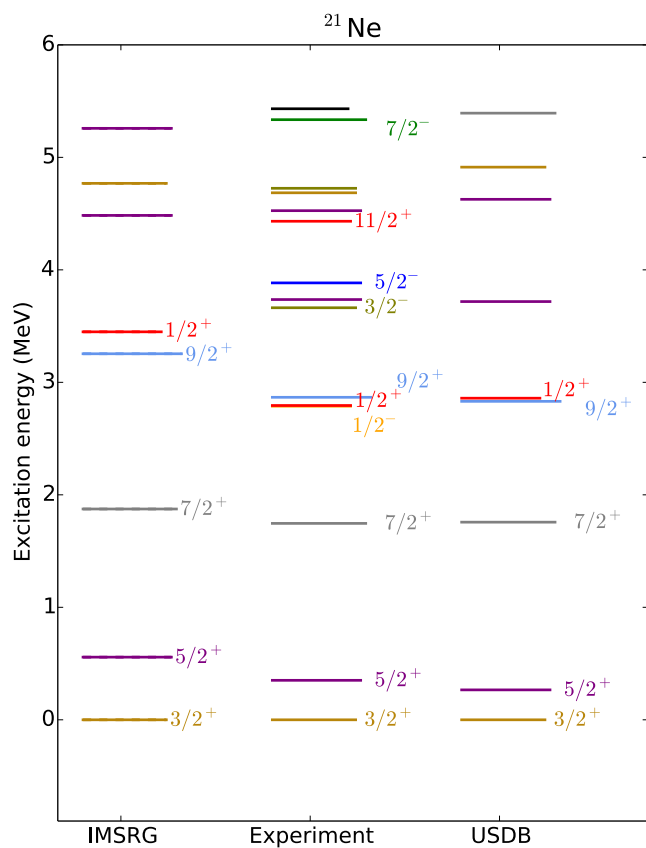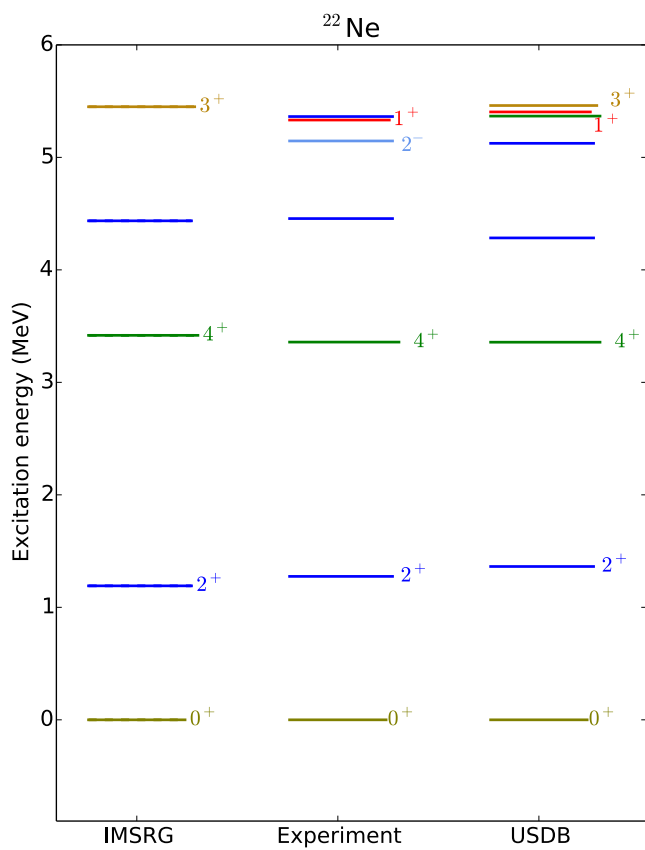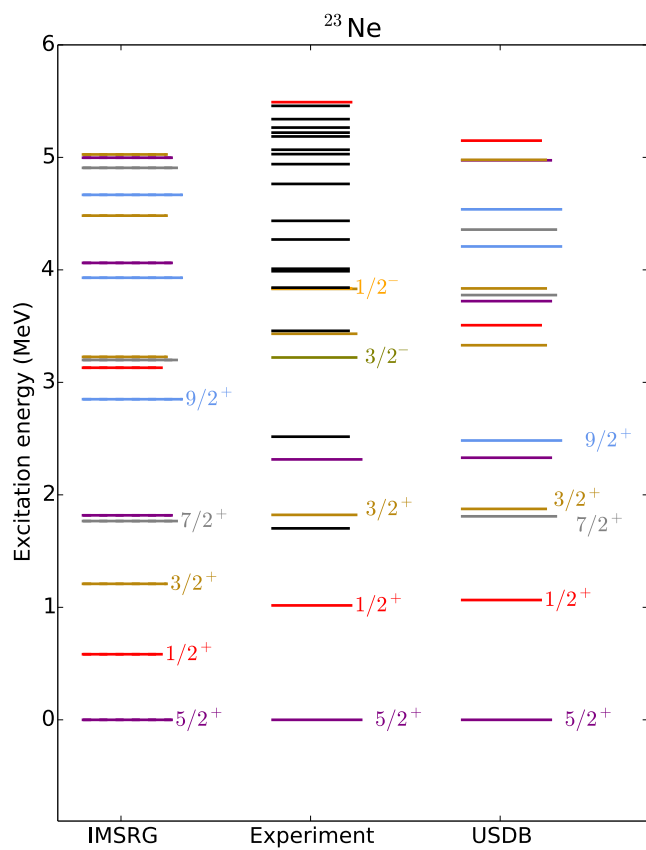



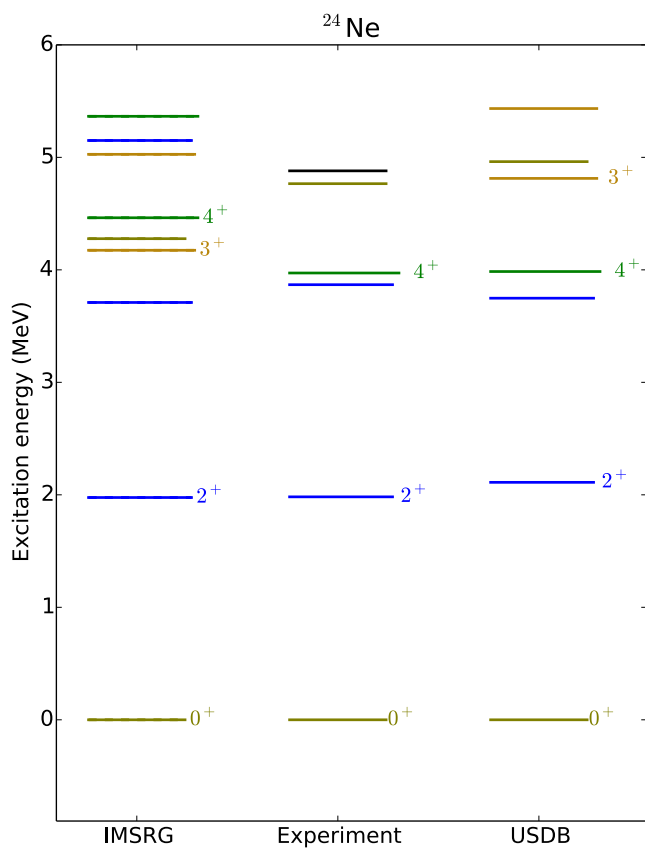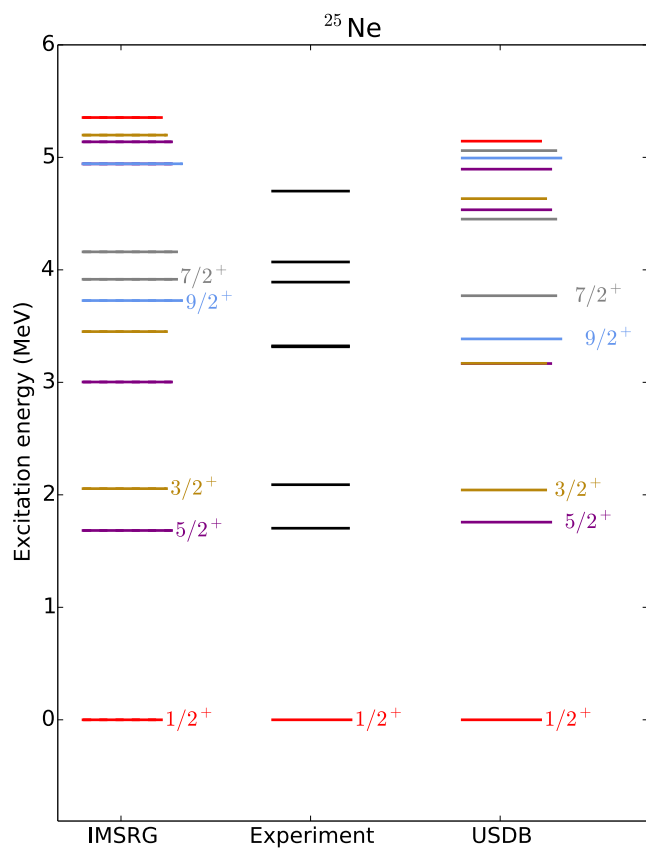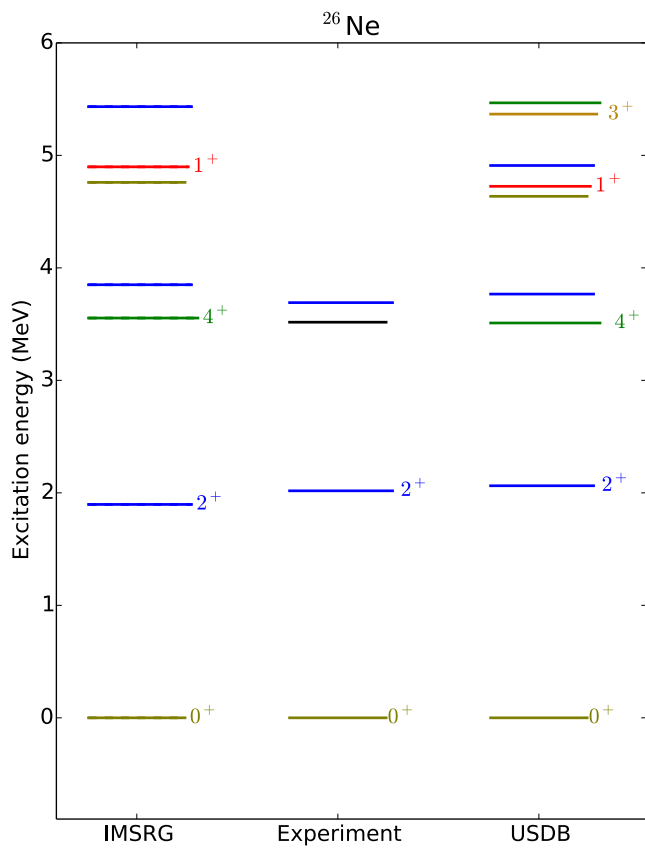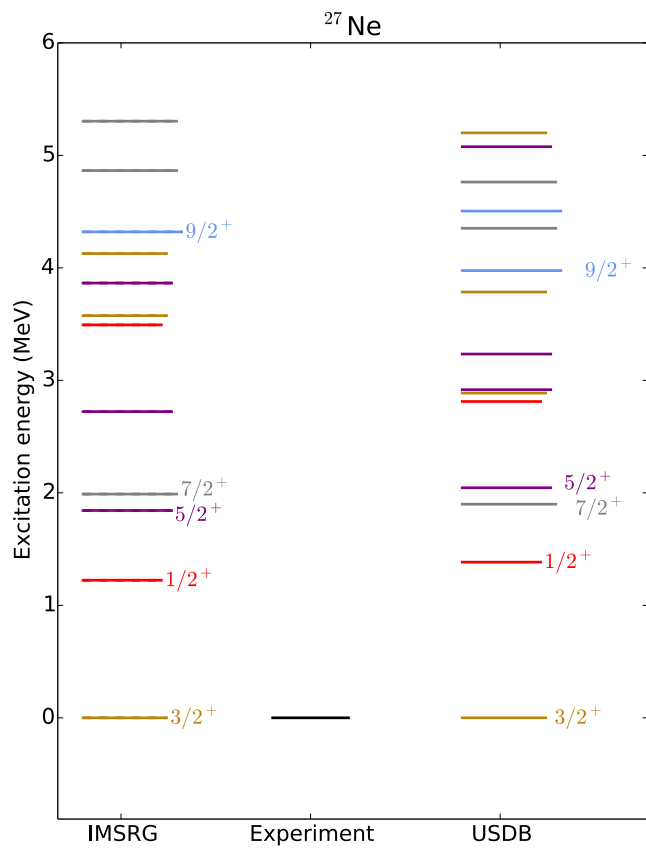

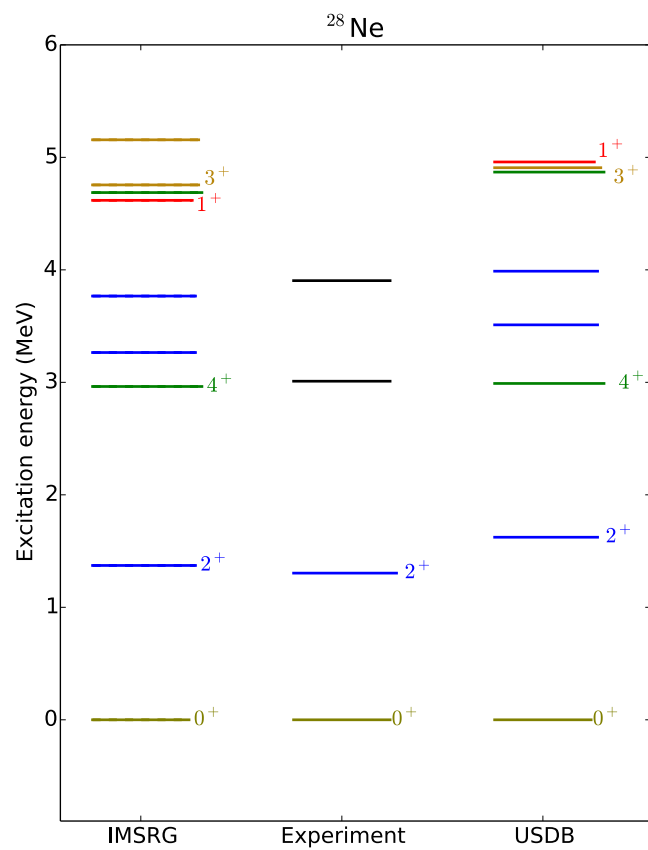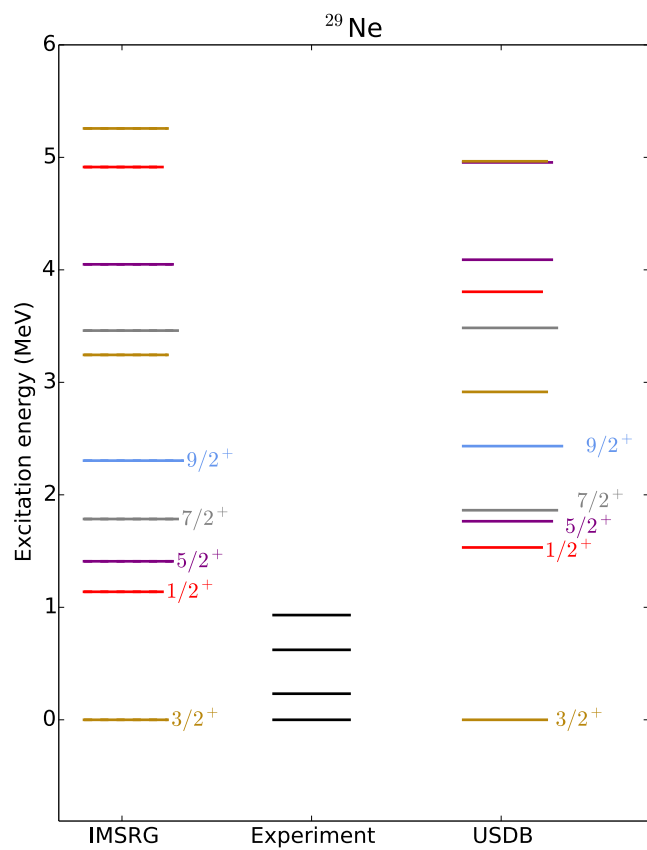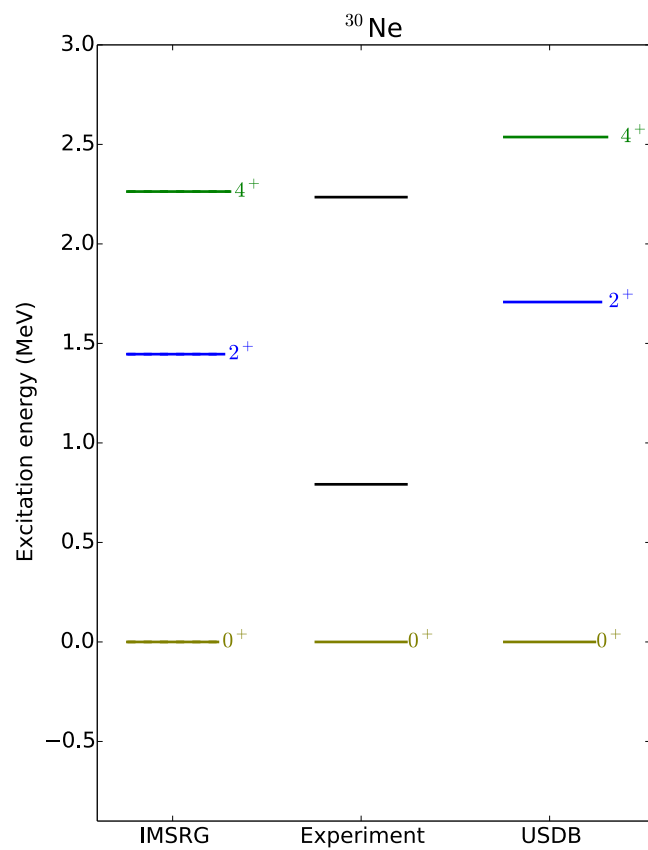

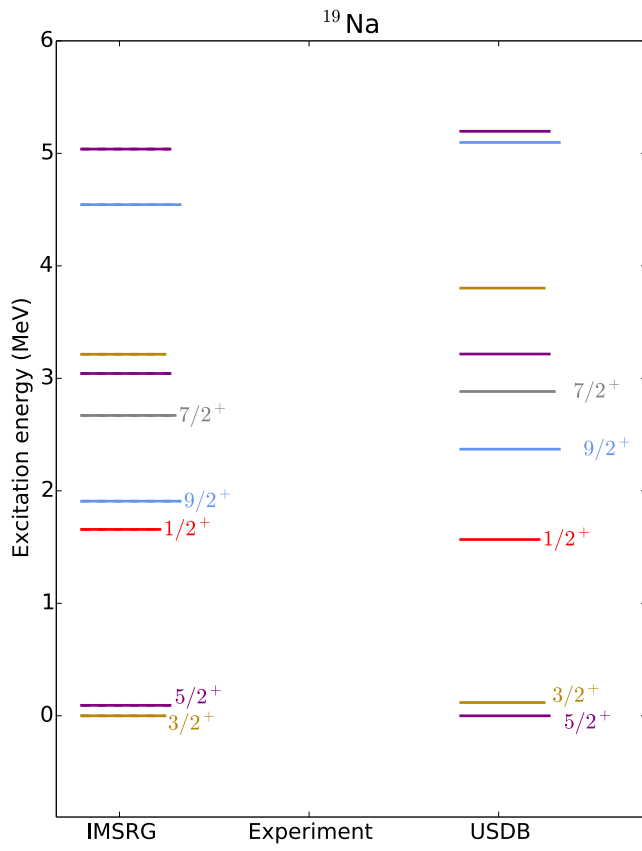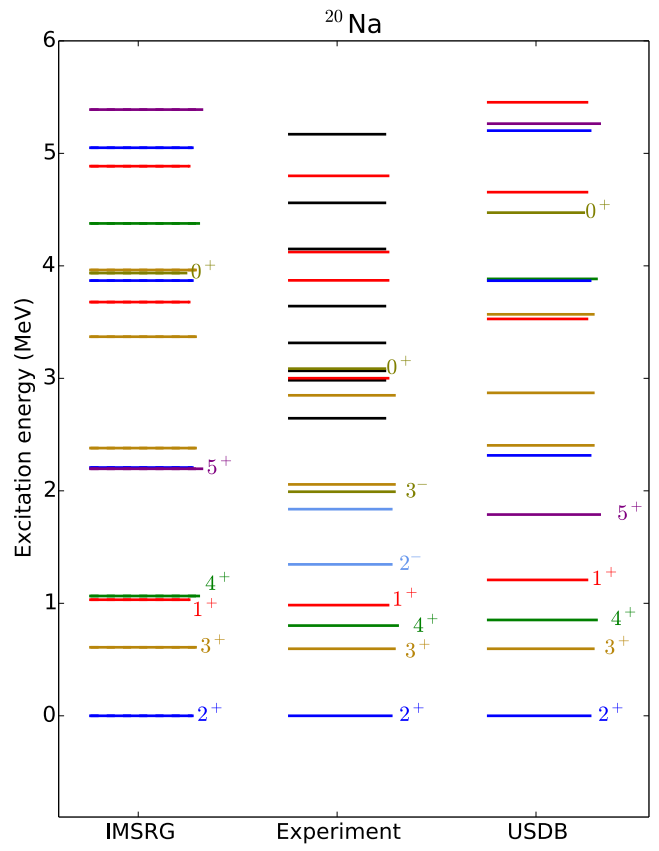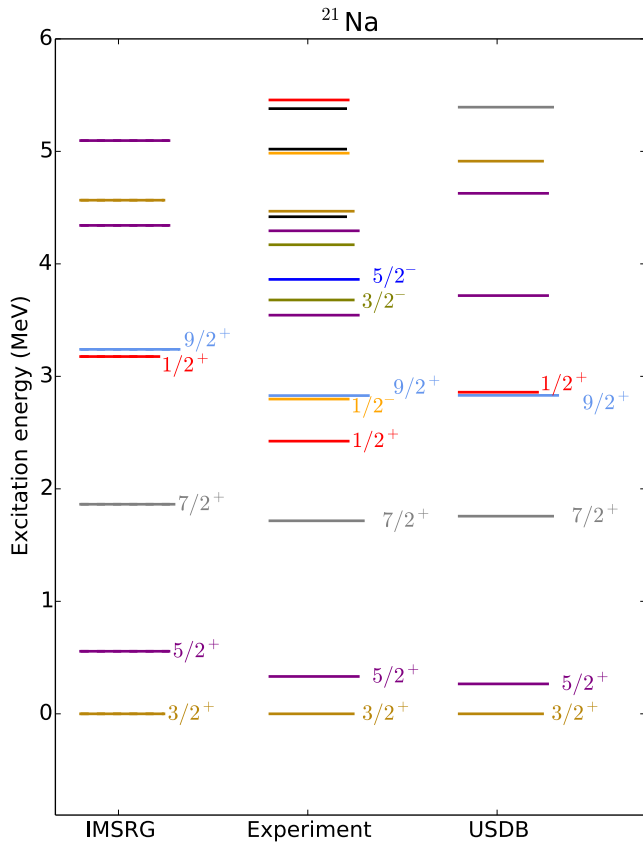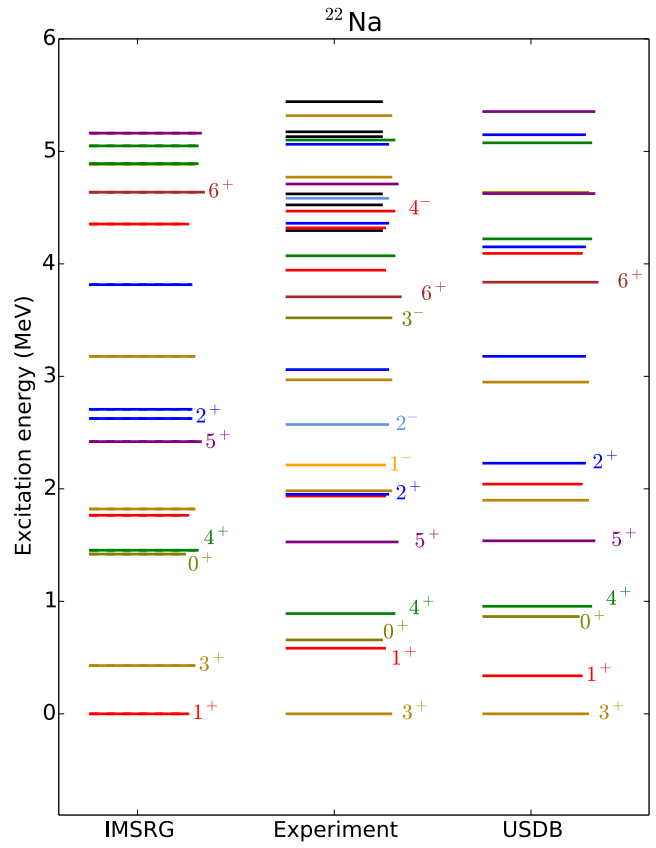

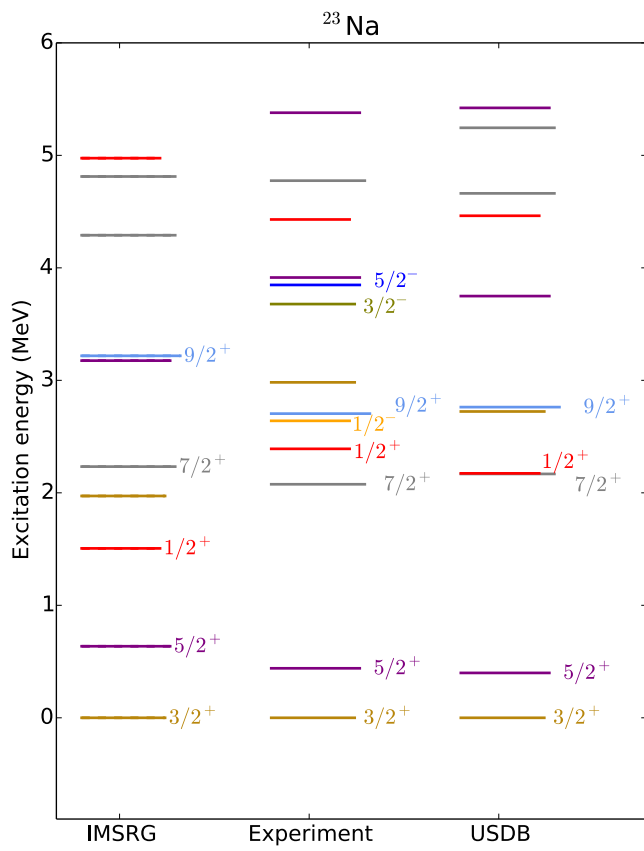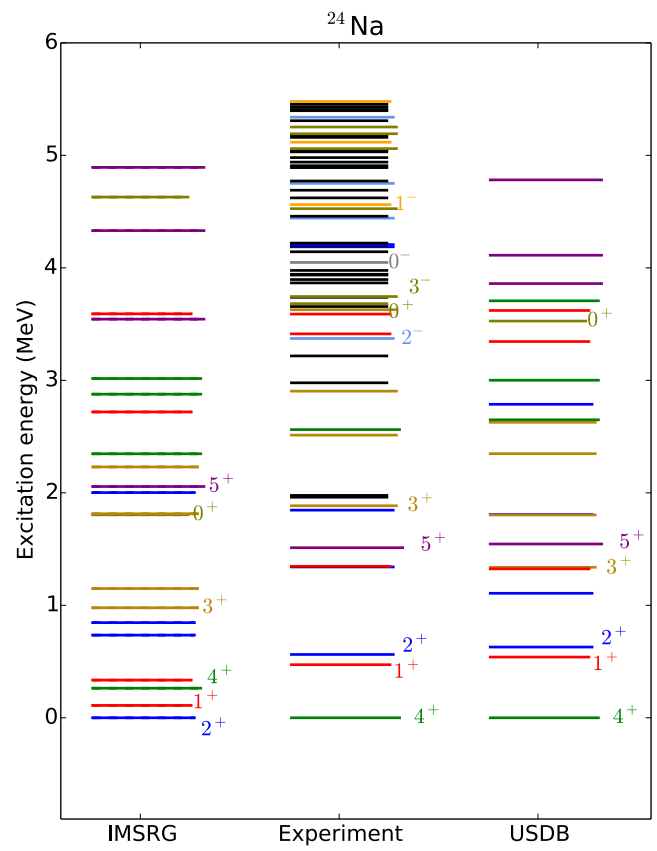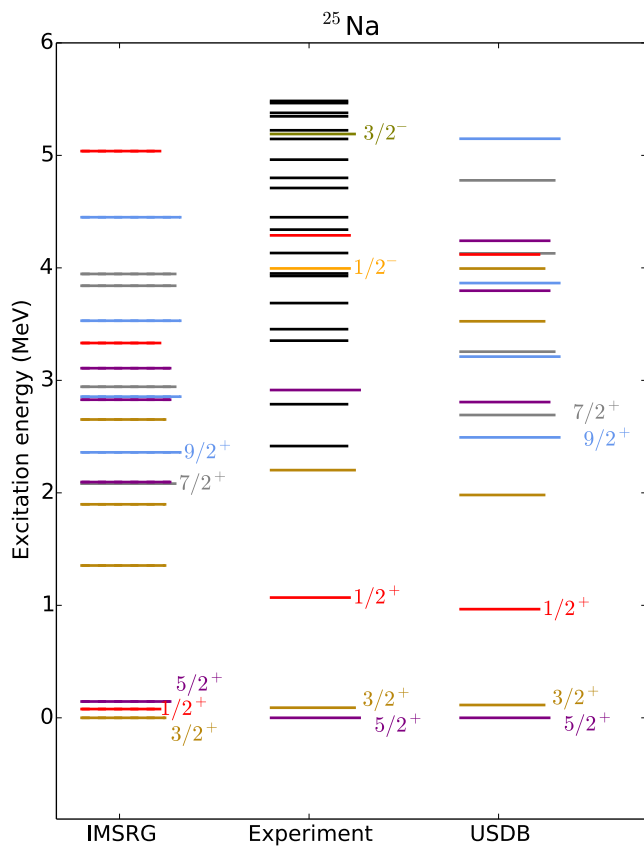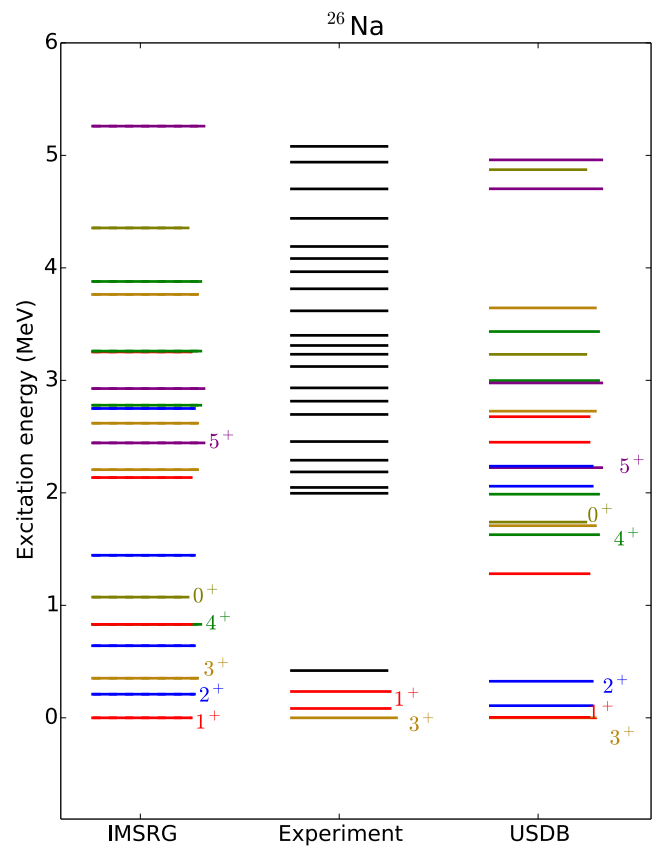

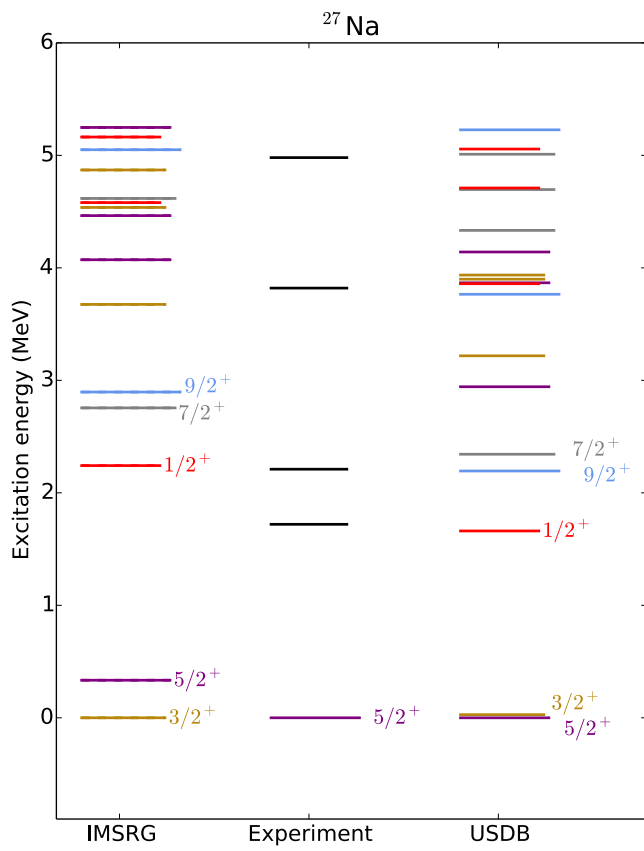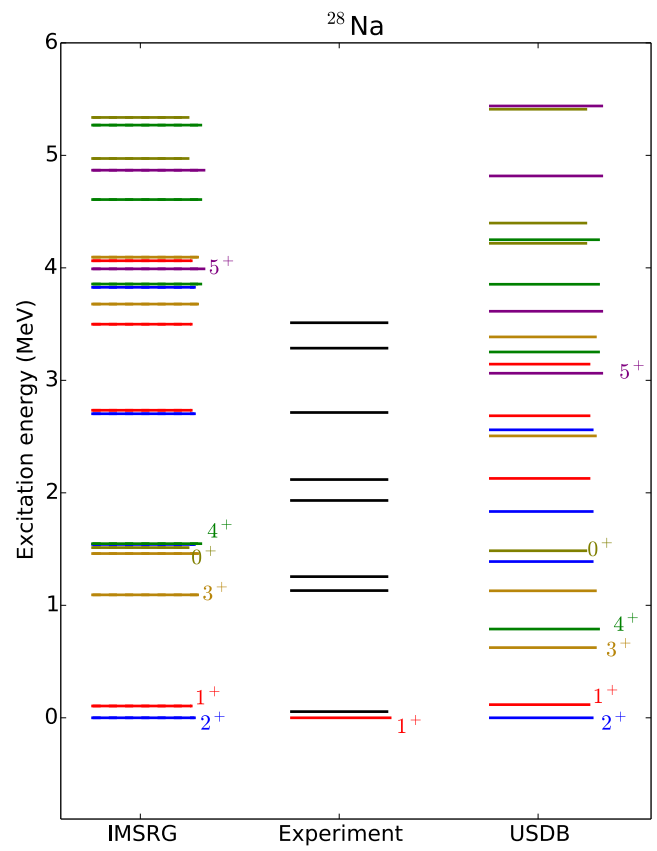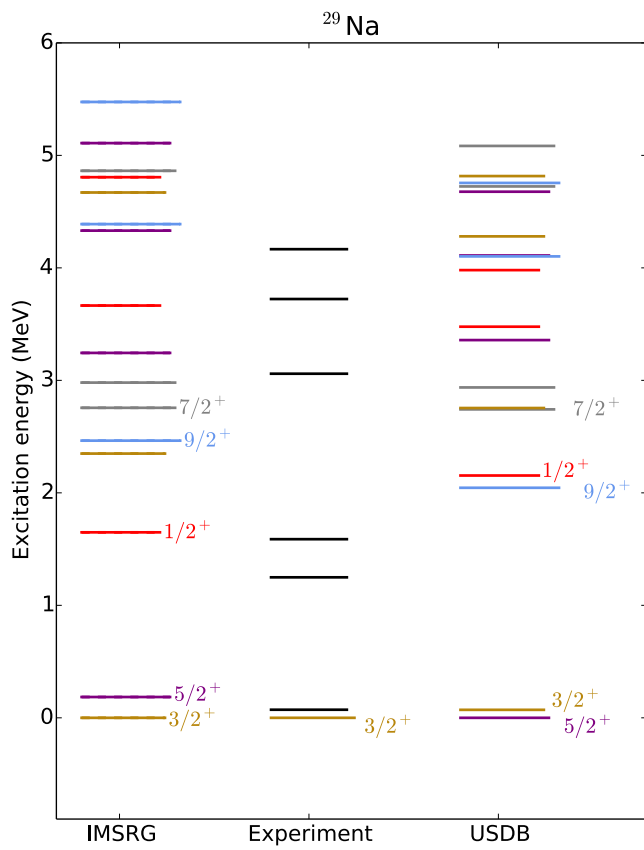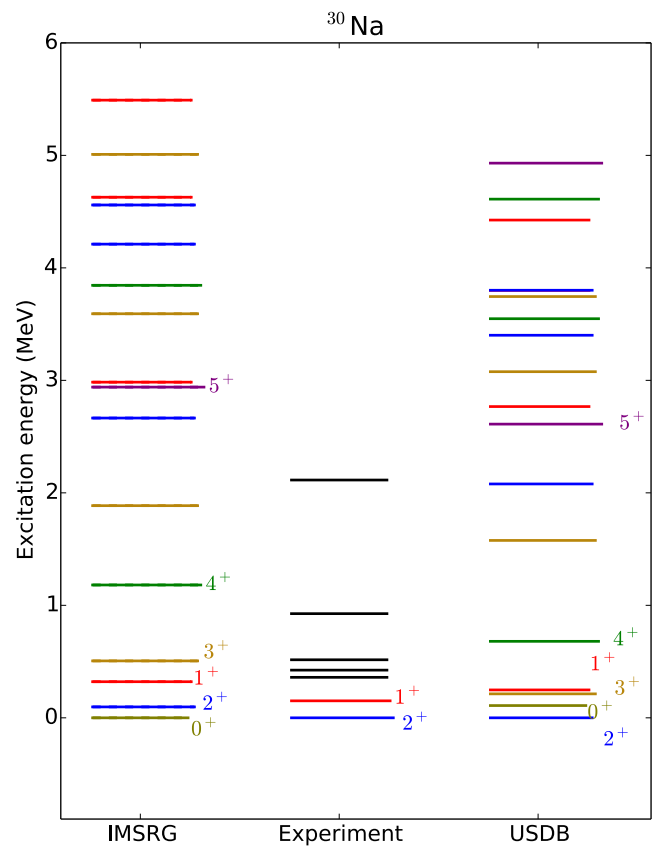

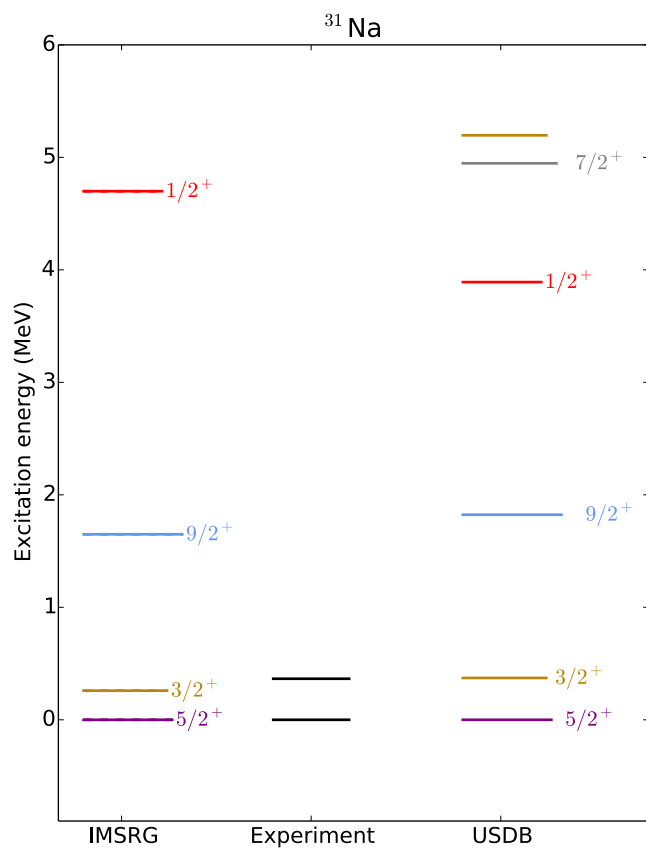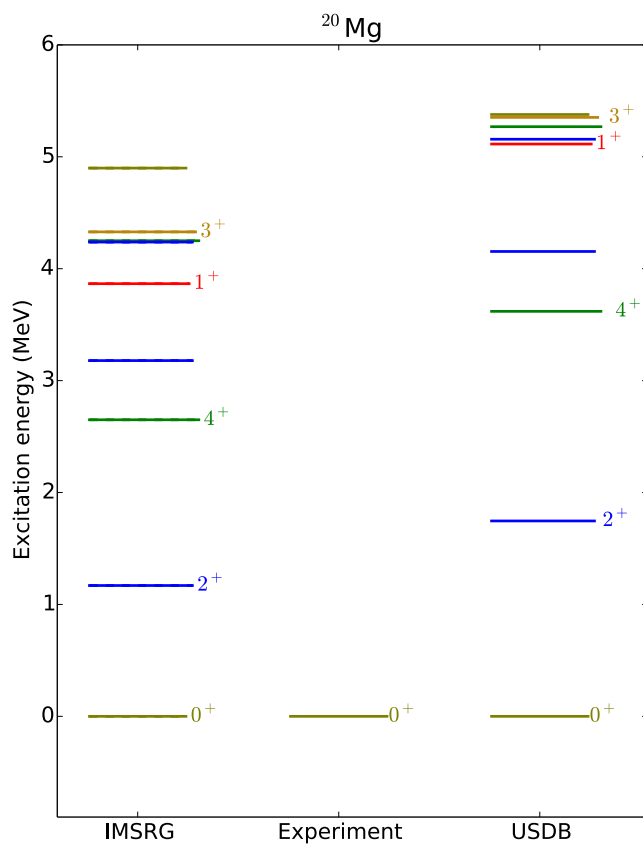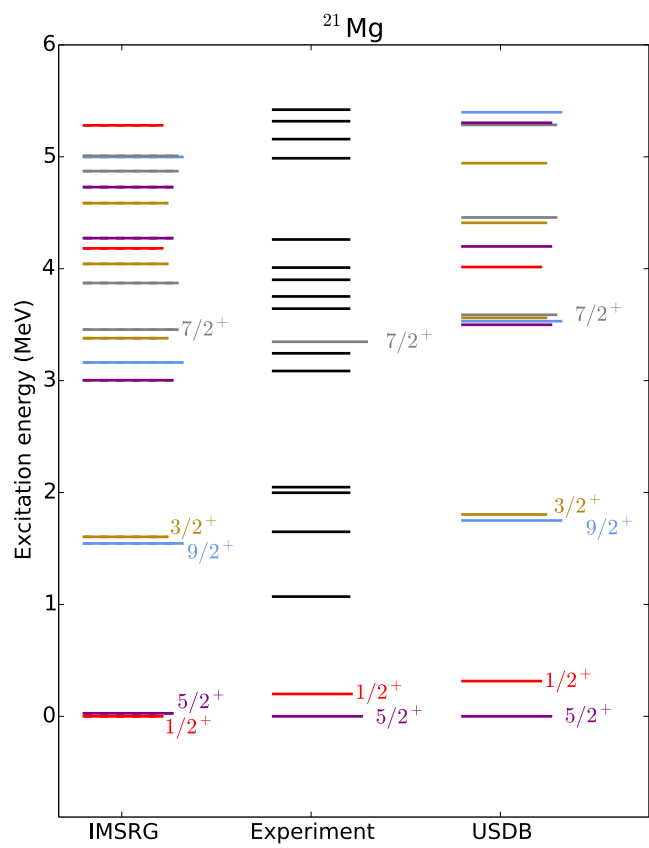

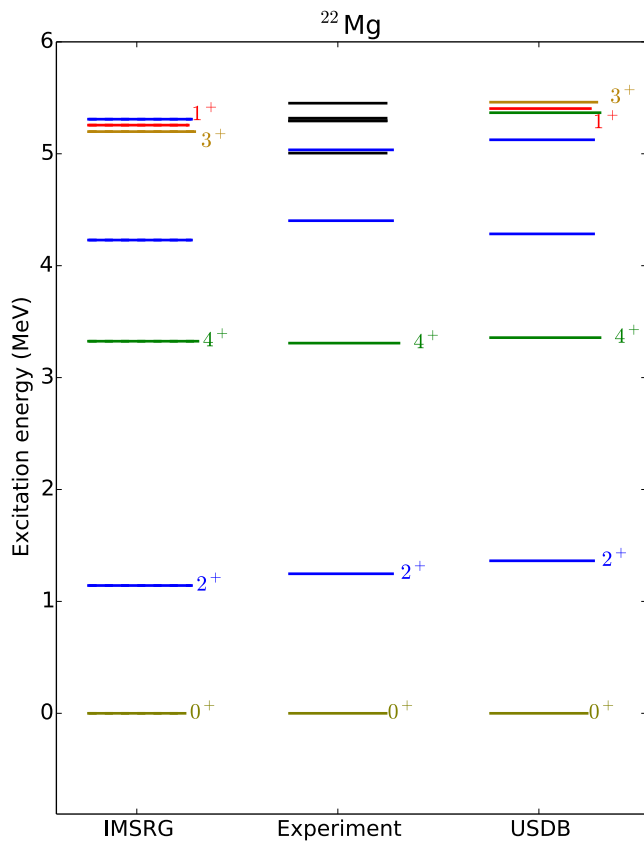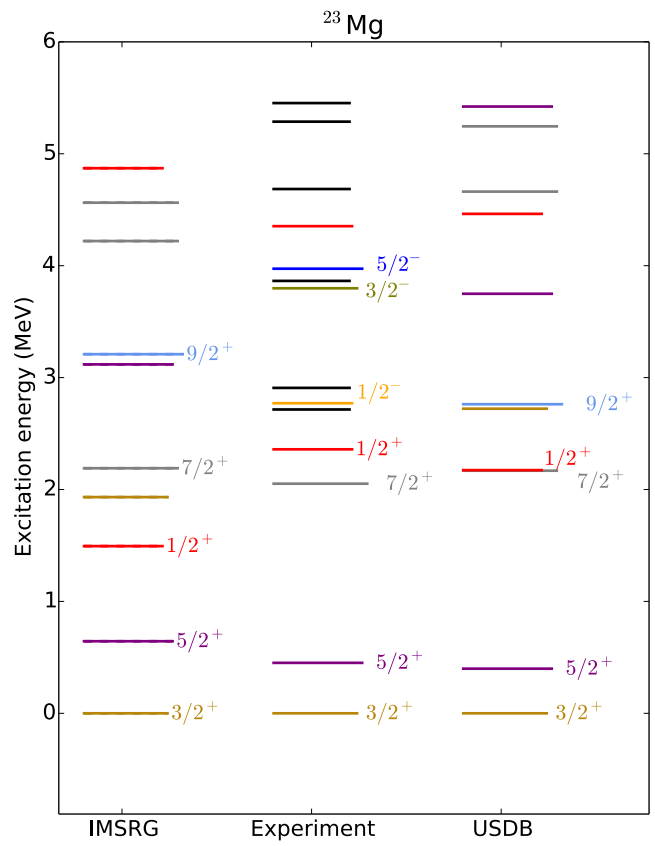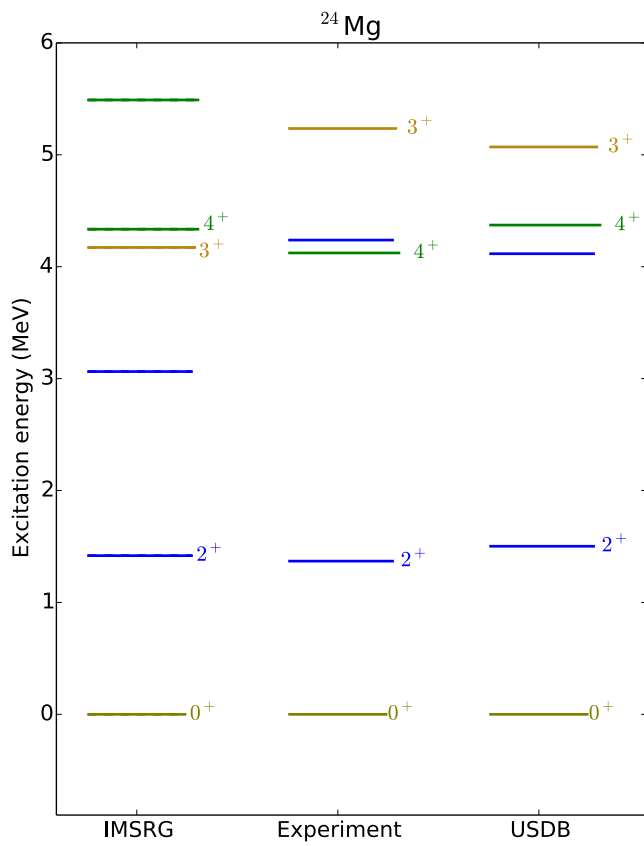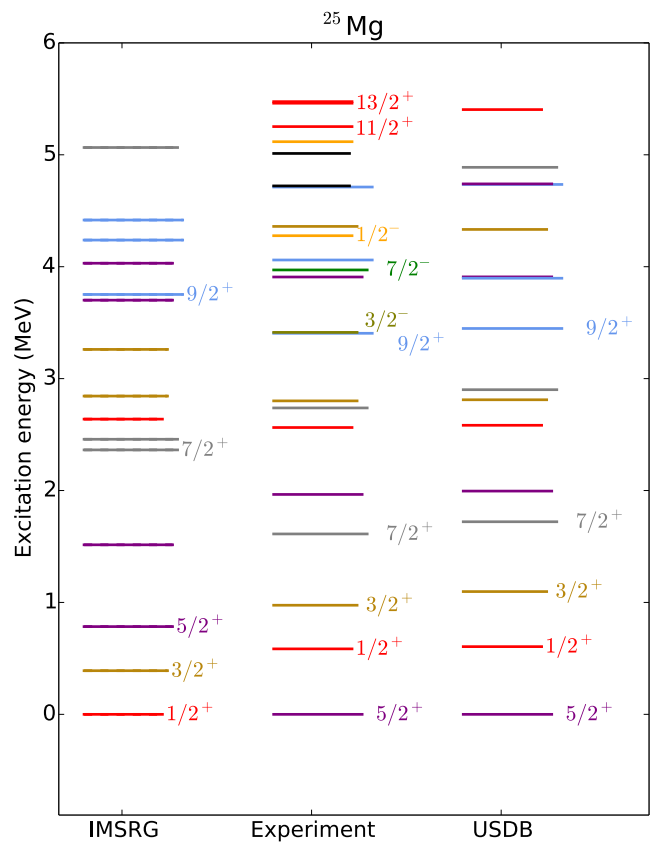

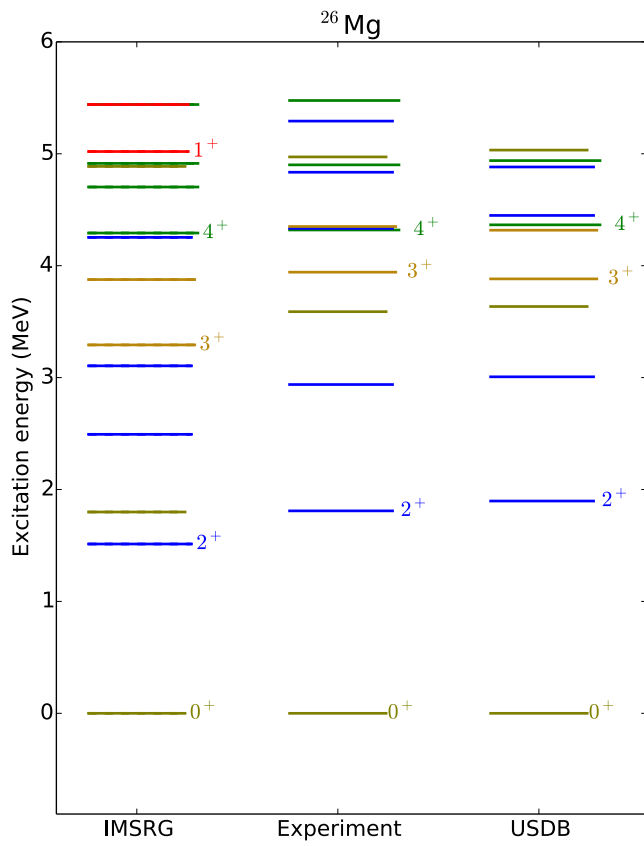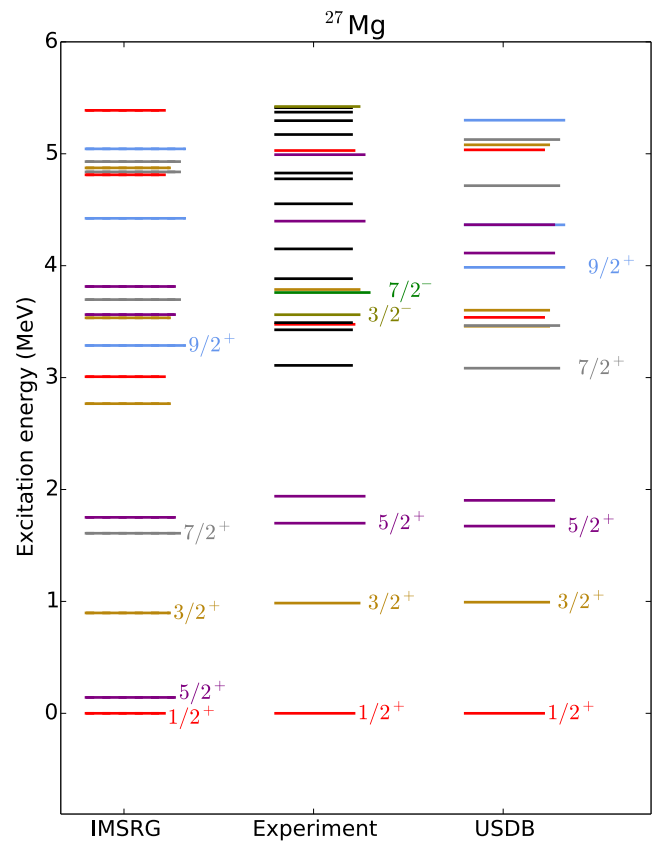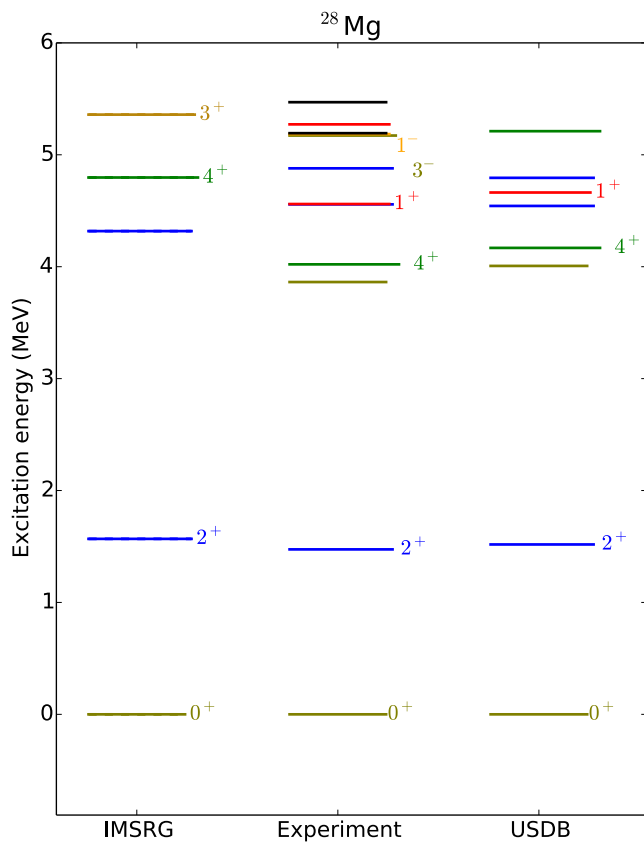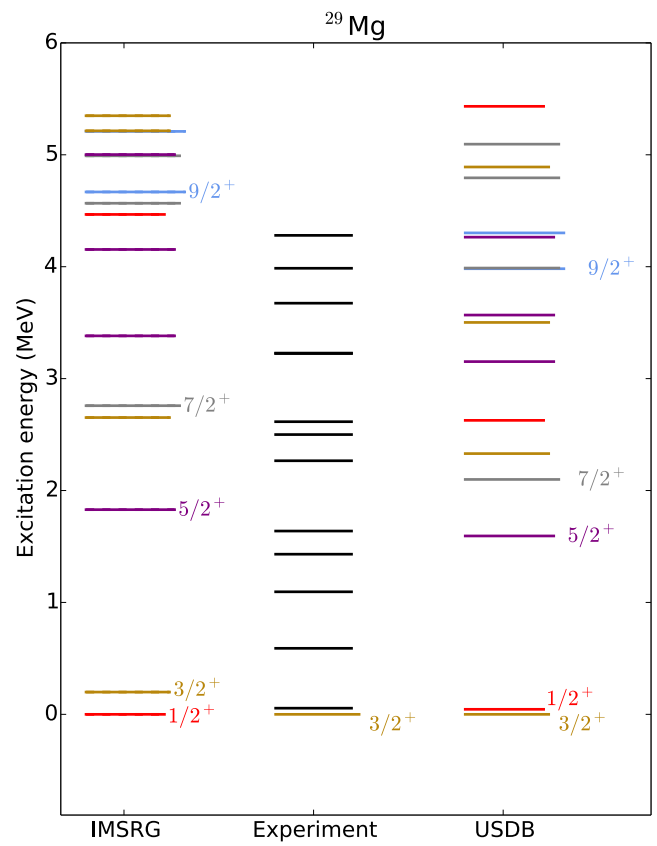



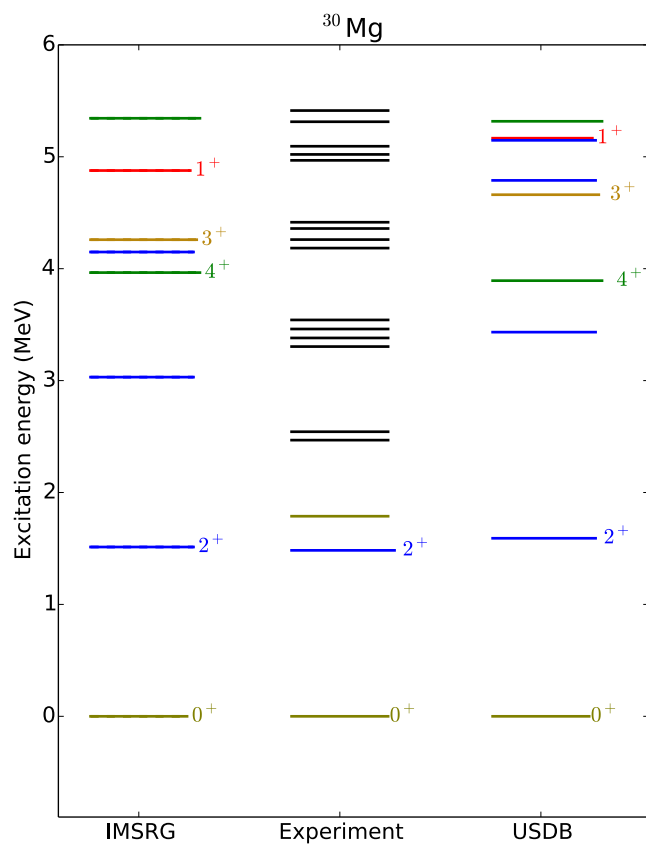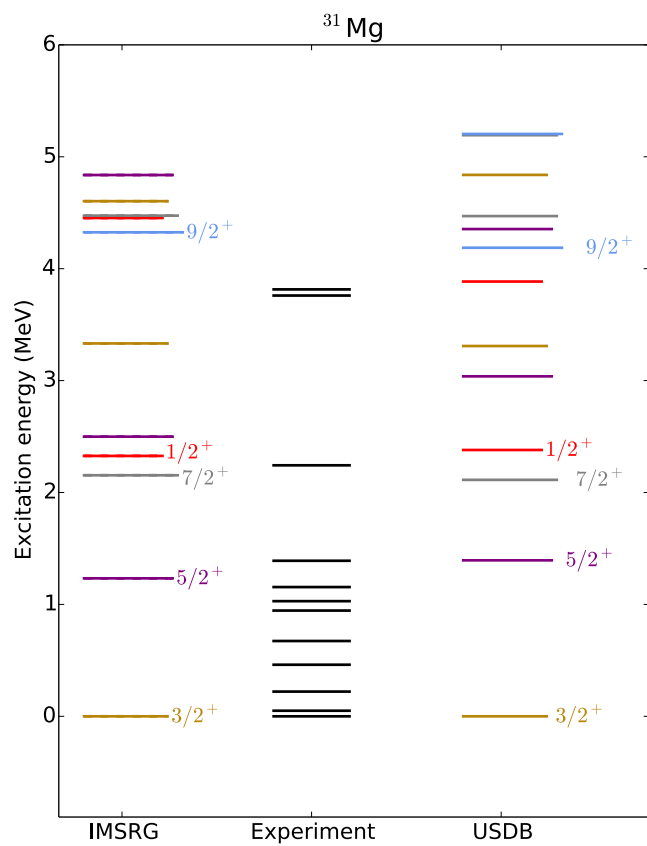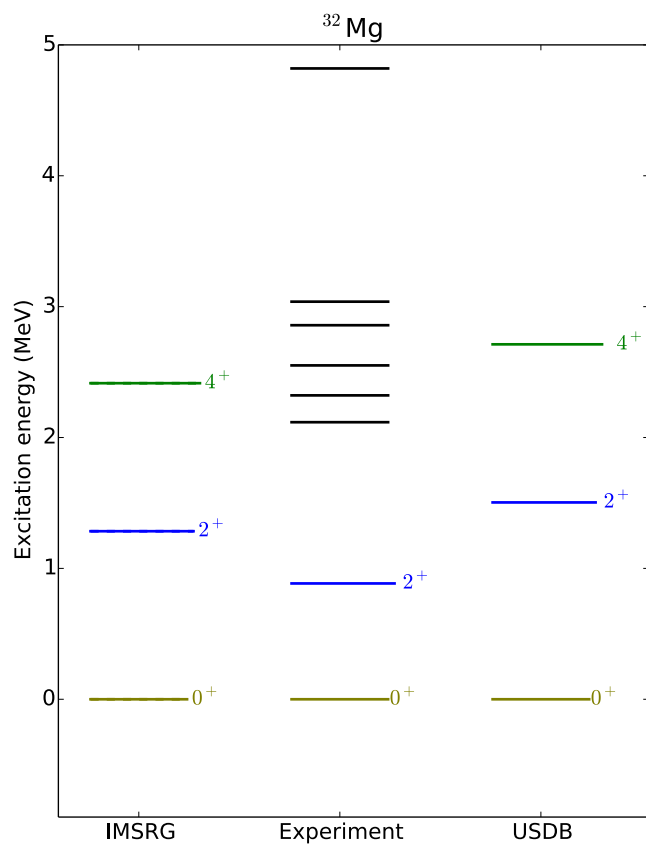

Supplement: Supplementary file 1 [file SupplementSpectra.pdf]
